# Supplementary material for: Simultaneous determination of CKM angle $\gamma$ and charm mixing parameters
Source: arXiv:2110.02350 source file (2022-01-07)
Supplement: Supplementary file 1 [file supplementary.tex]

\section*{Supplementary Information}
%\section{Supplemental material}
\label{sec:Supplementary}

%Should be sent in PDF format
%Should all be referenced in the main text as e.g. Supplementary Fig. X
%Submitted as a separate file and must have independent numbering

\setcounter{figure}{0}
\setcounter{table}{0}

%Some additional content we would like to provide.
%Credible intervals from Bayesian analysis are provided in Supplementary Table~\ref{tab:Dh_combBayes}.
%A demonstration of the improvement in charm parameters from performing the simultaneous average in Supplementary Fig.~\ref{fig:res:charm_pars}.
A breakdown of the contributing components in the combination shown in Supplementary Fig.~\ref{fig:res:breakdown_2d_dh}. A summary of LHCb \g combination results as a function of time is given in Supplementary Fig.~\ref{fig:gammaevolution}.

\begin{table}[!tb]
  \centering
    \caption{Credibility regions and most probable values for the hadronic parameters extracted from the \g combination using Bayesian inference.}
    \begin{tabular}{lccc}
    \hline
    Quantity & Value & \multicolumn{2}{c}{Credibility Intervals (Bayesian)}\\
	        & 		& 68.3\% 	&95.4\%  \\
    \hline
    $\g [^{\circ}]$     & 65.6 & [61.8,69.3] & [58.0,72.6] \\
    $\dbdk [^{\circ}]$  & 127.8 & [123.9,131.7] & [119.9,135.2] \\
    $\dbdpi [^{\circ}]$ & 290 & [276,302] & [262,313] \\
    $\rbdk$             & 0.0989 & [0.0964,0.1014] & [0.0939,0.1039] \\
    $\rbdpi$            & 0.00487 & [0.00429,0.00551] & [0.00381,0.00625] \\
     \hline
    \end{tabular}
    \label{tab:Dh_combBayes}
\end{table}

\begin{figure}[!tb]
  \centering
  \includegraphics[width=0.48\textwidth]{figs/gammacharm_lhcb_comp_rD_kpi.pdf}
  \includegraphics[width=0.48\textwidth]{figs/gammacharm_lhcb_comp_dD_kpi.pdf} \\
  \includegraphics[width=0.48\textwidth]{figs/gammacharm_lhcb_comp_xD.pdf}
  \includegraphics[width=0.48\textwidth]{figs/gammacharm_lhcb_comp_yD.pdf} \\
  \includegraphics[width=0.48\textwidth]{figs/gammacharm_lhcb_comp_qopD.pdf}
  \includegraphics[width=0.48\textwidth]{figs/gammacharm_lhcb_comp_phiD.pdf}
  \caption{The \omcl distributions for each of the parameters relating to the charm part of the average. }
  \label{fig:res:charm_pars}
\end{figure}

\begin{figure}[!tb]
  \centering
  \includegraphics[width=0.48\textwidth]{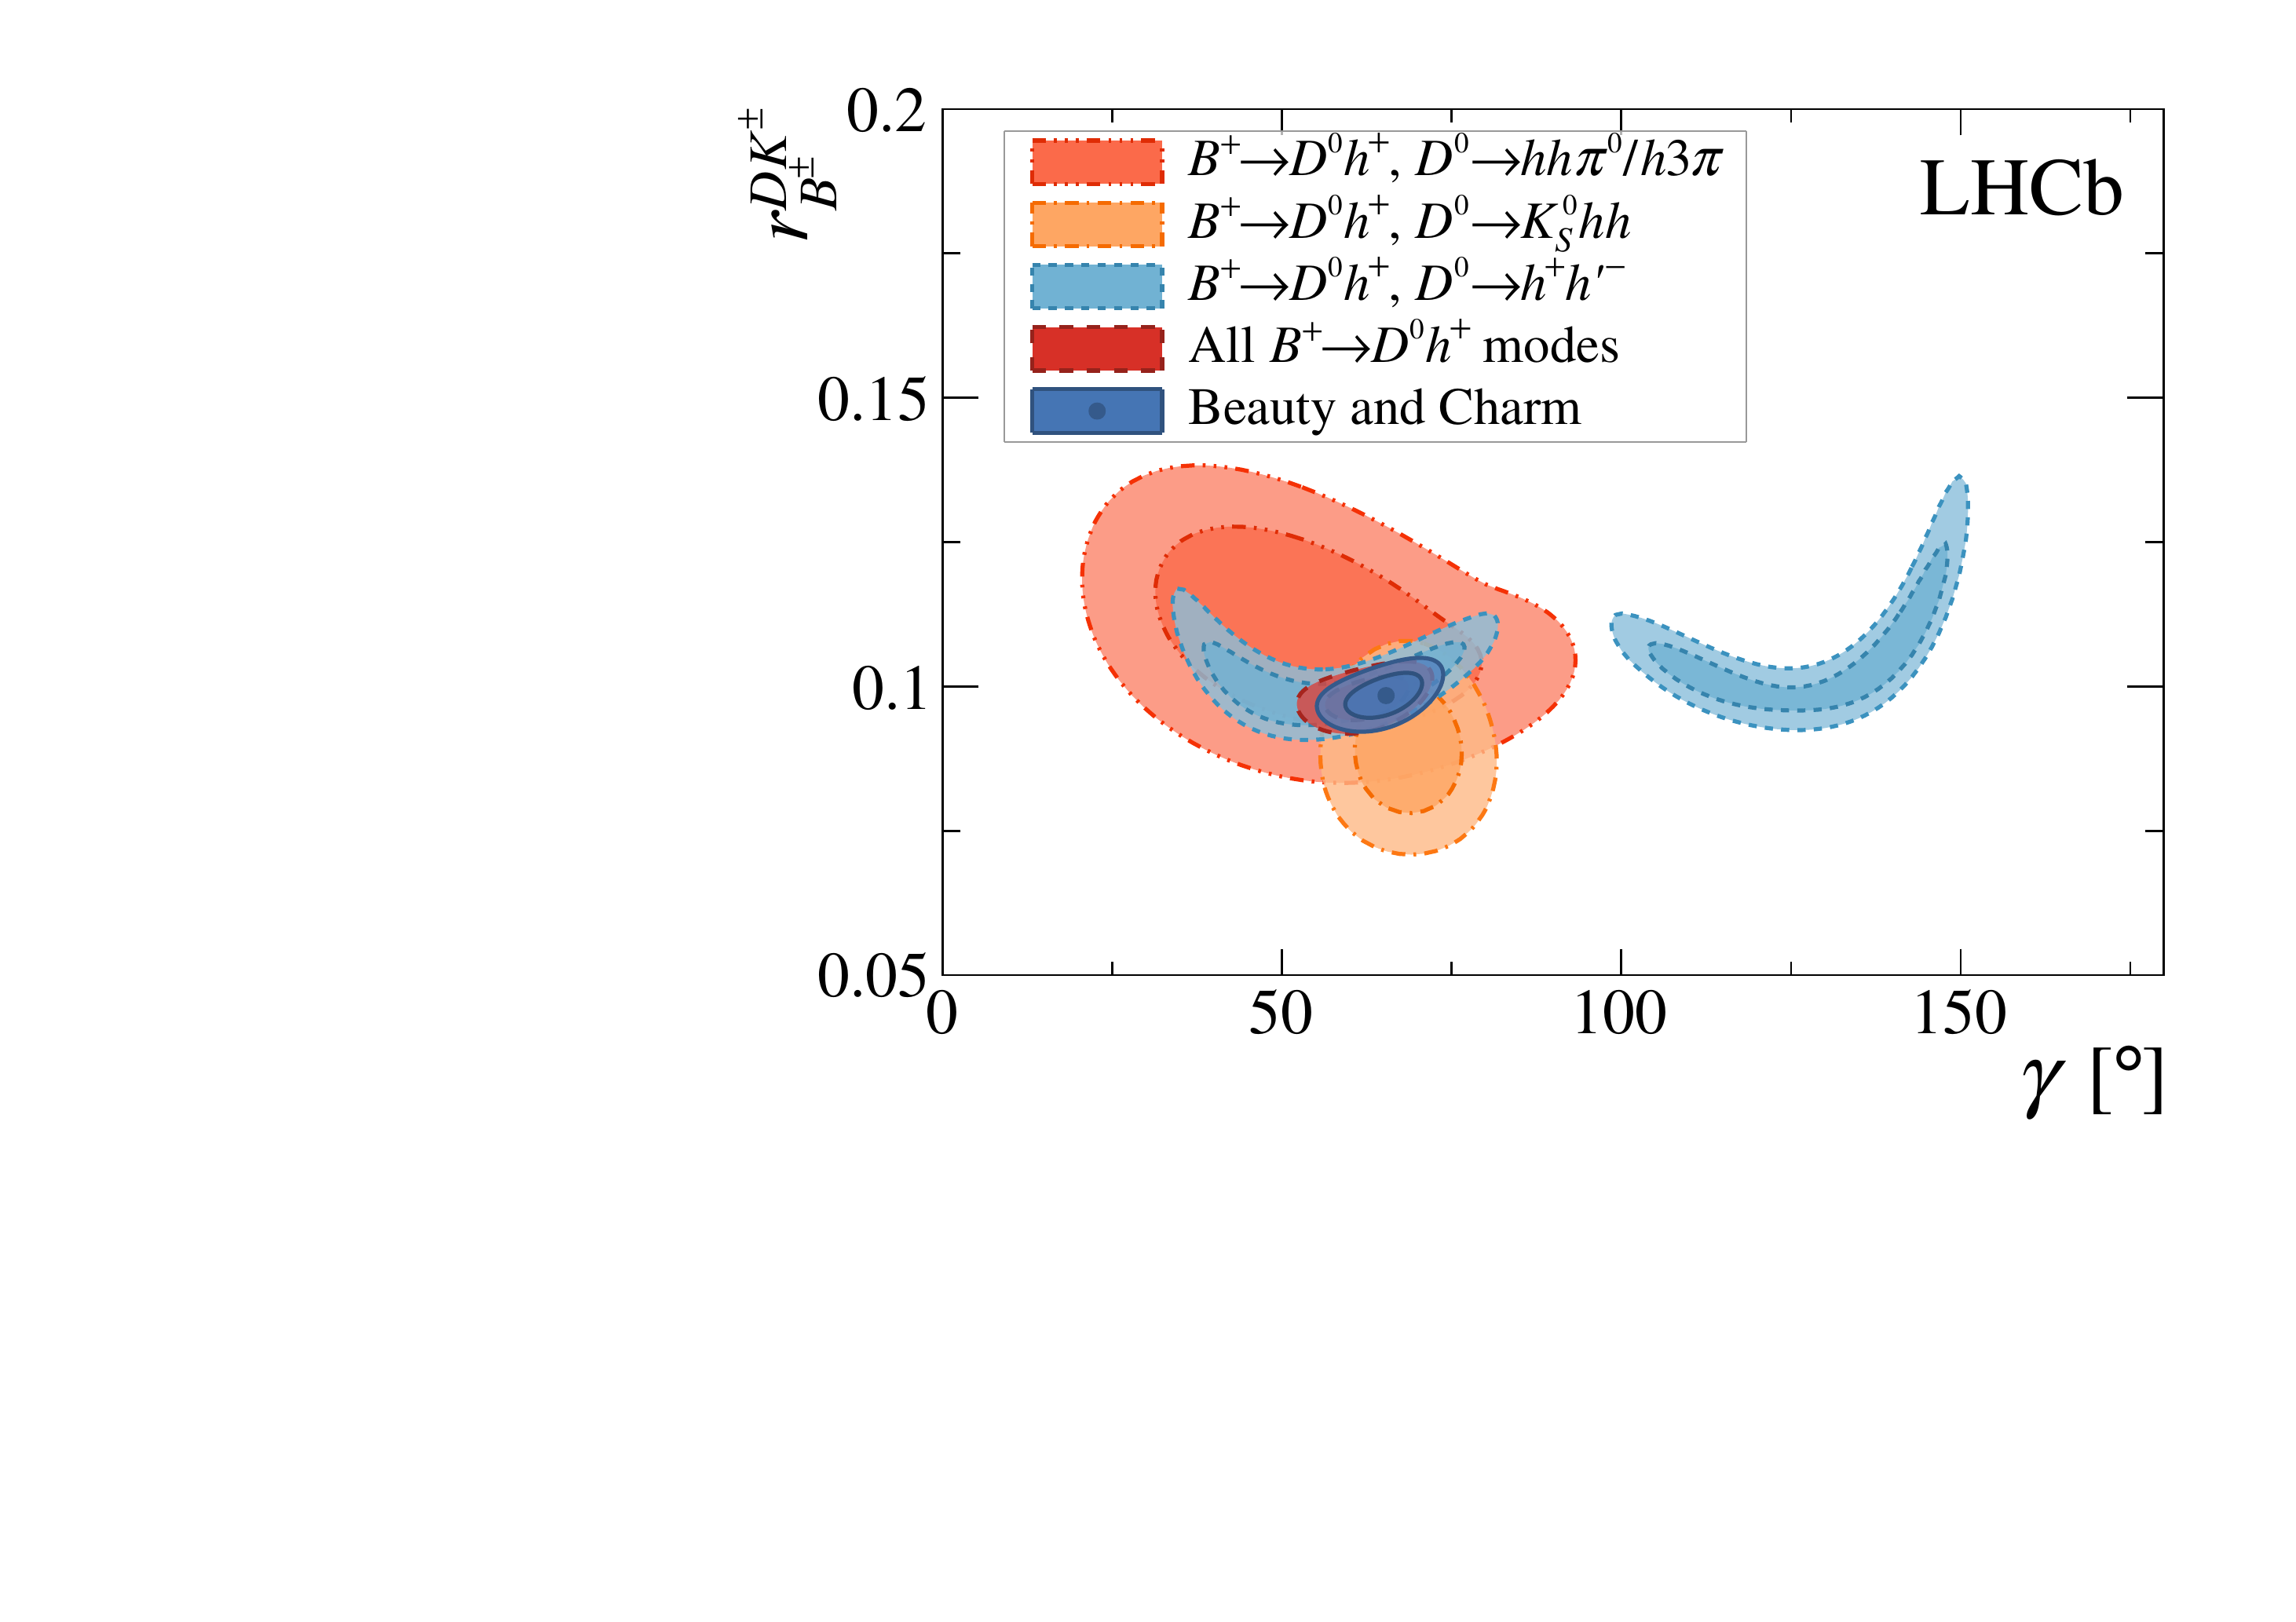}
  \includegraphics[width=0.48\textwidth]{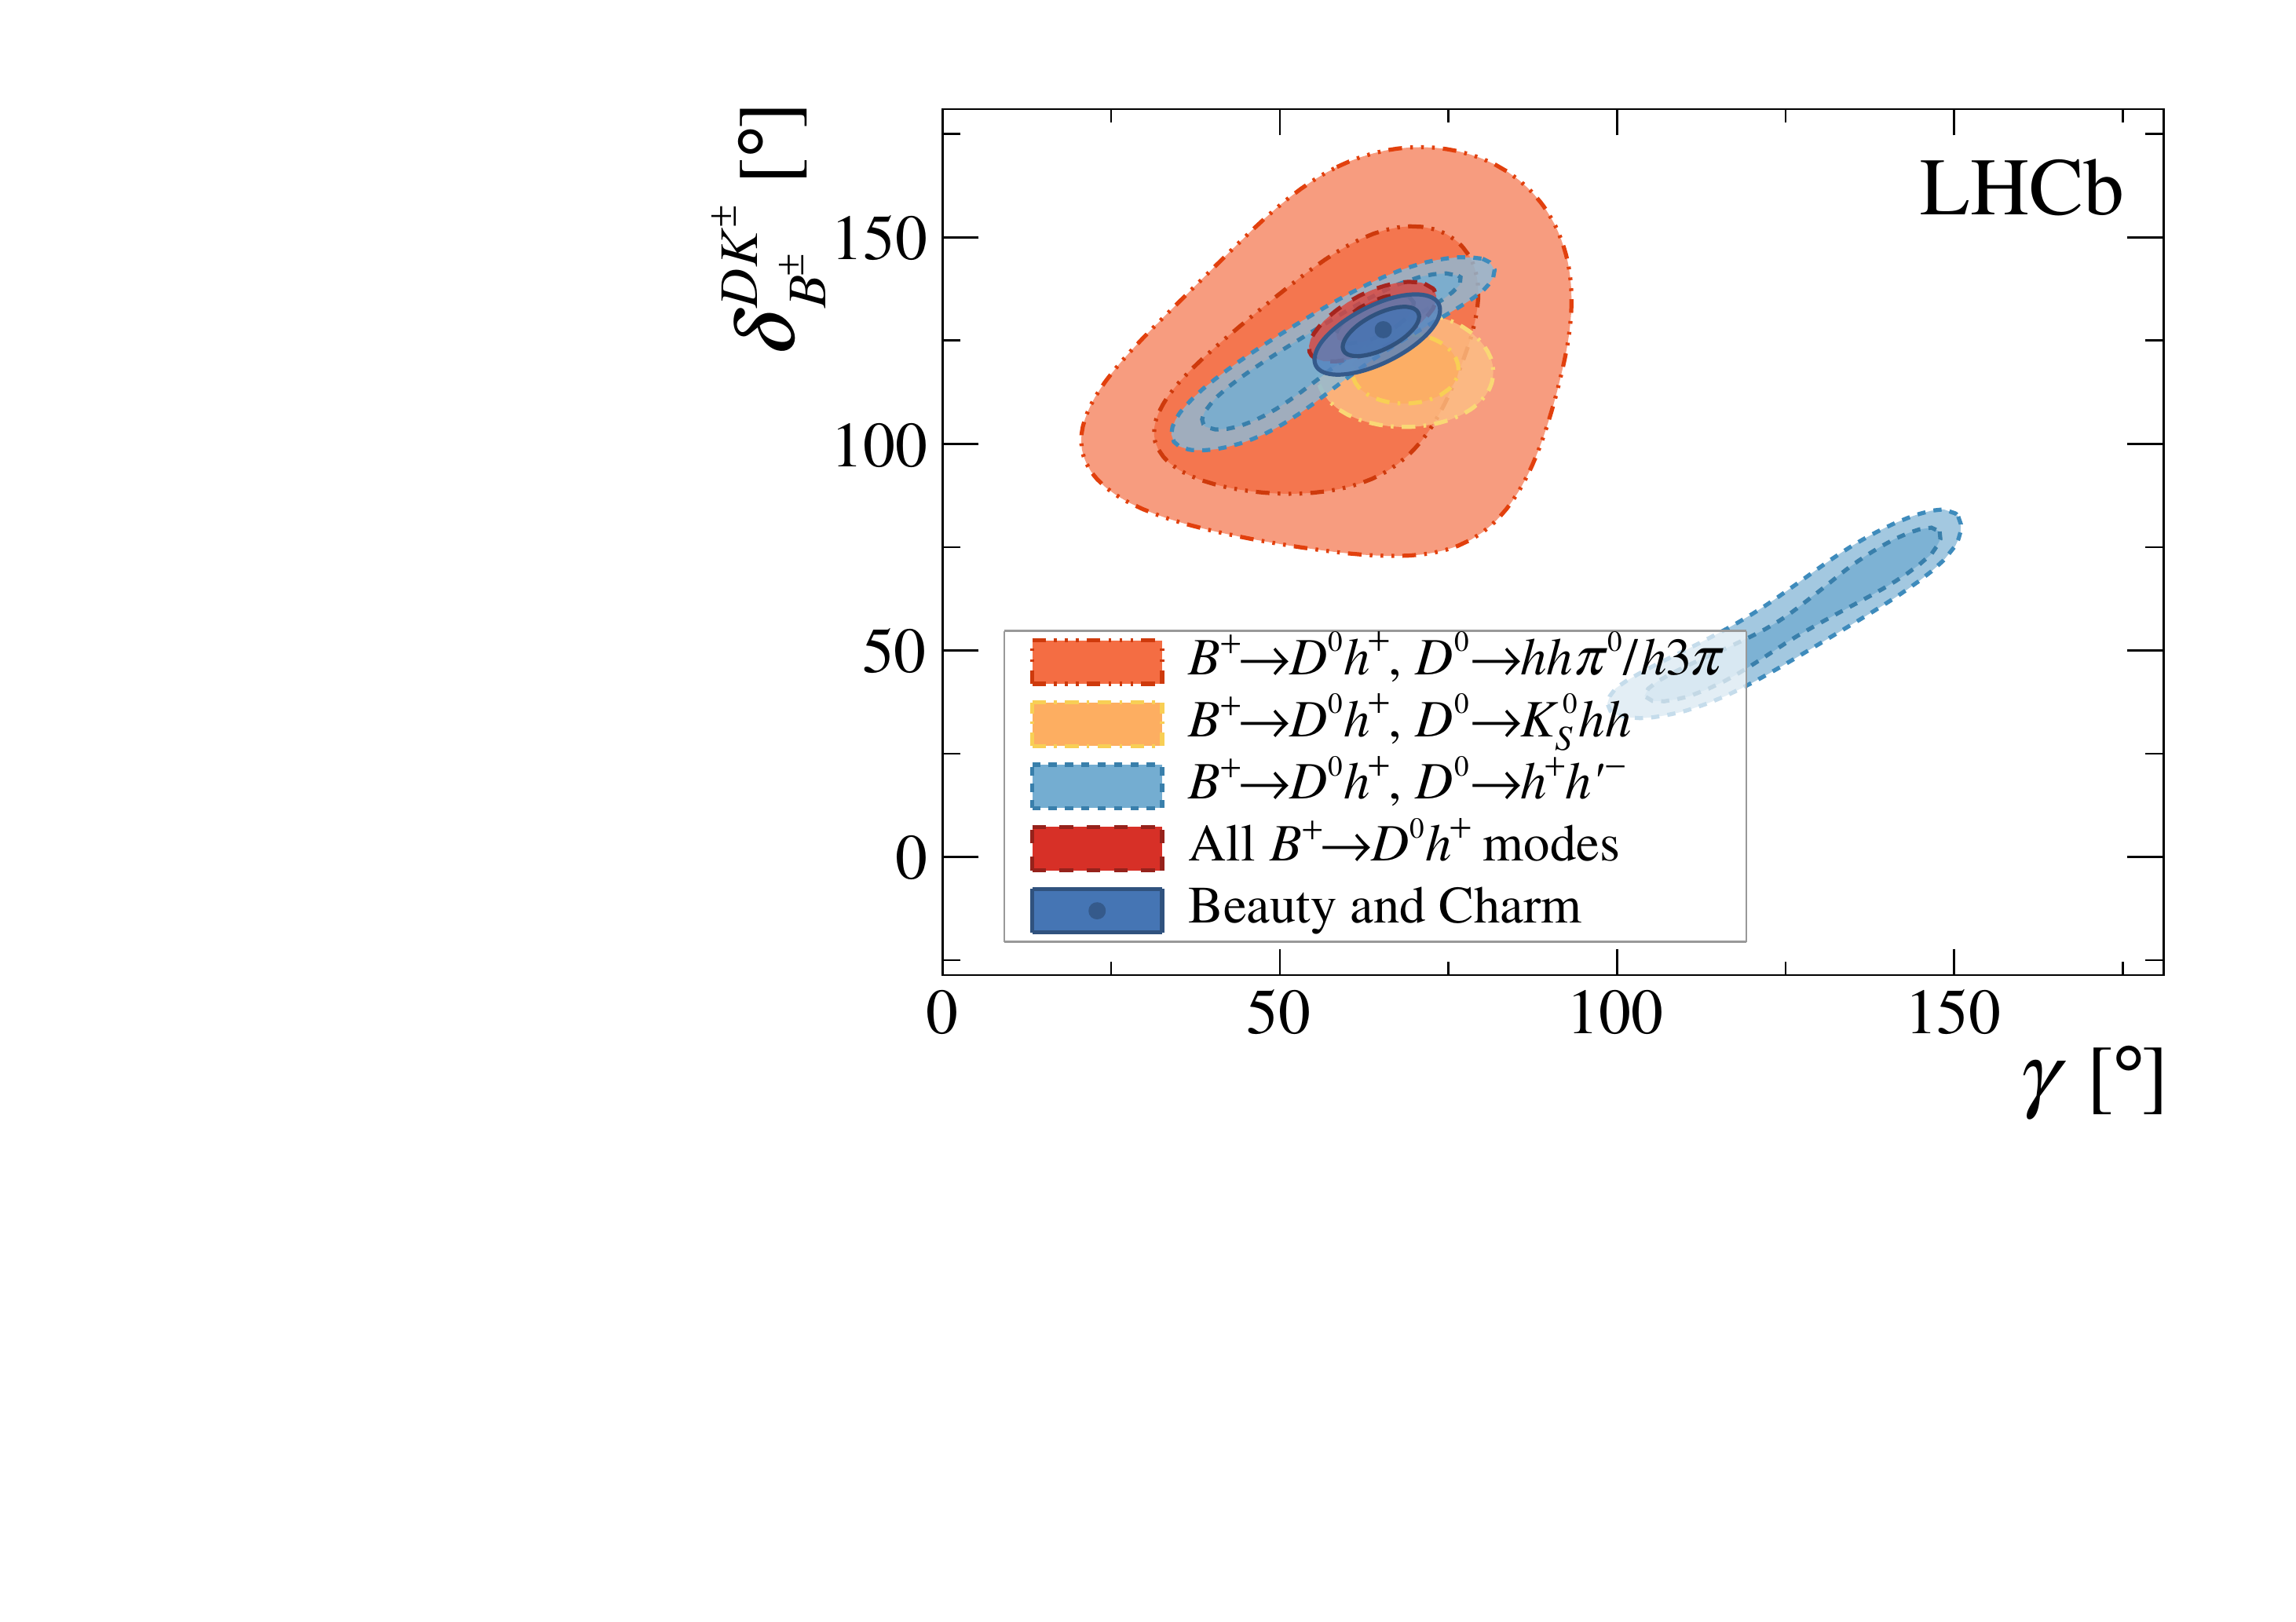}
  \includegraphics[width=0.48\textwidth]{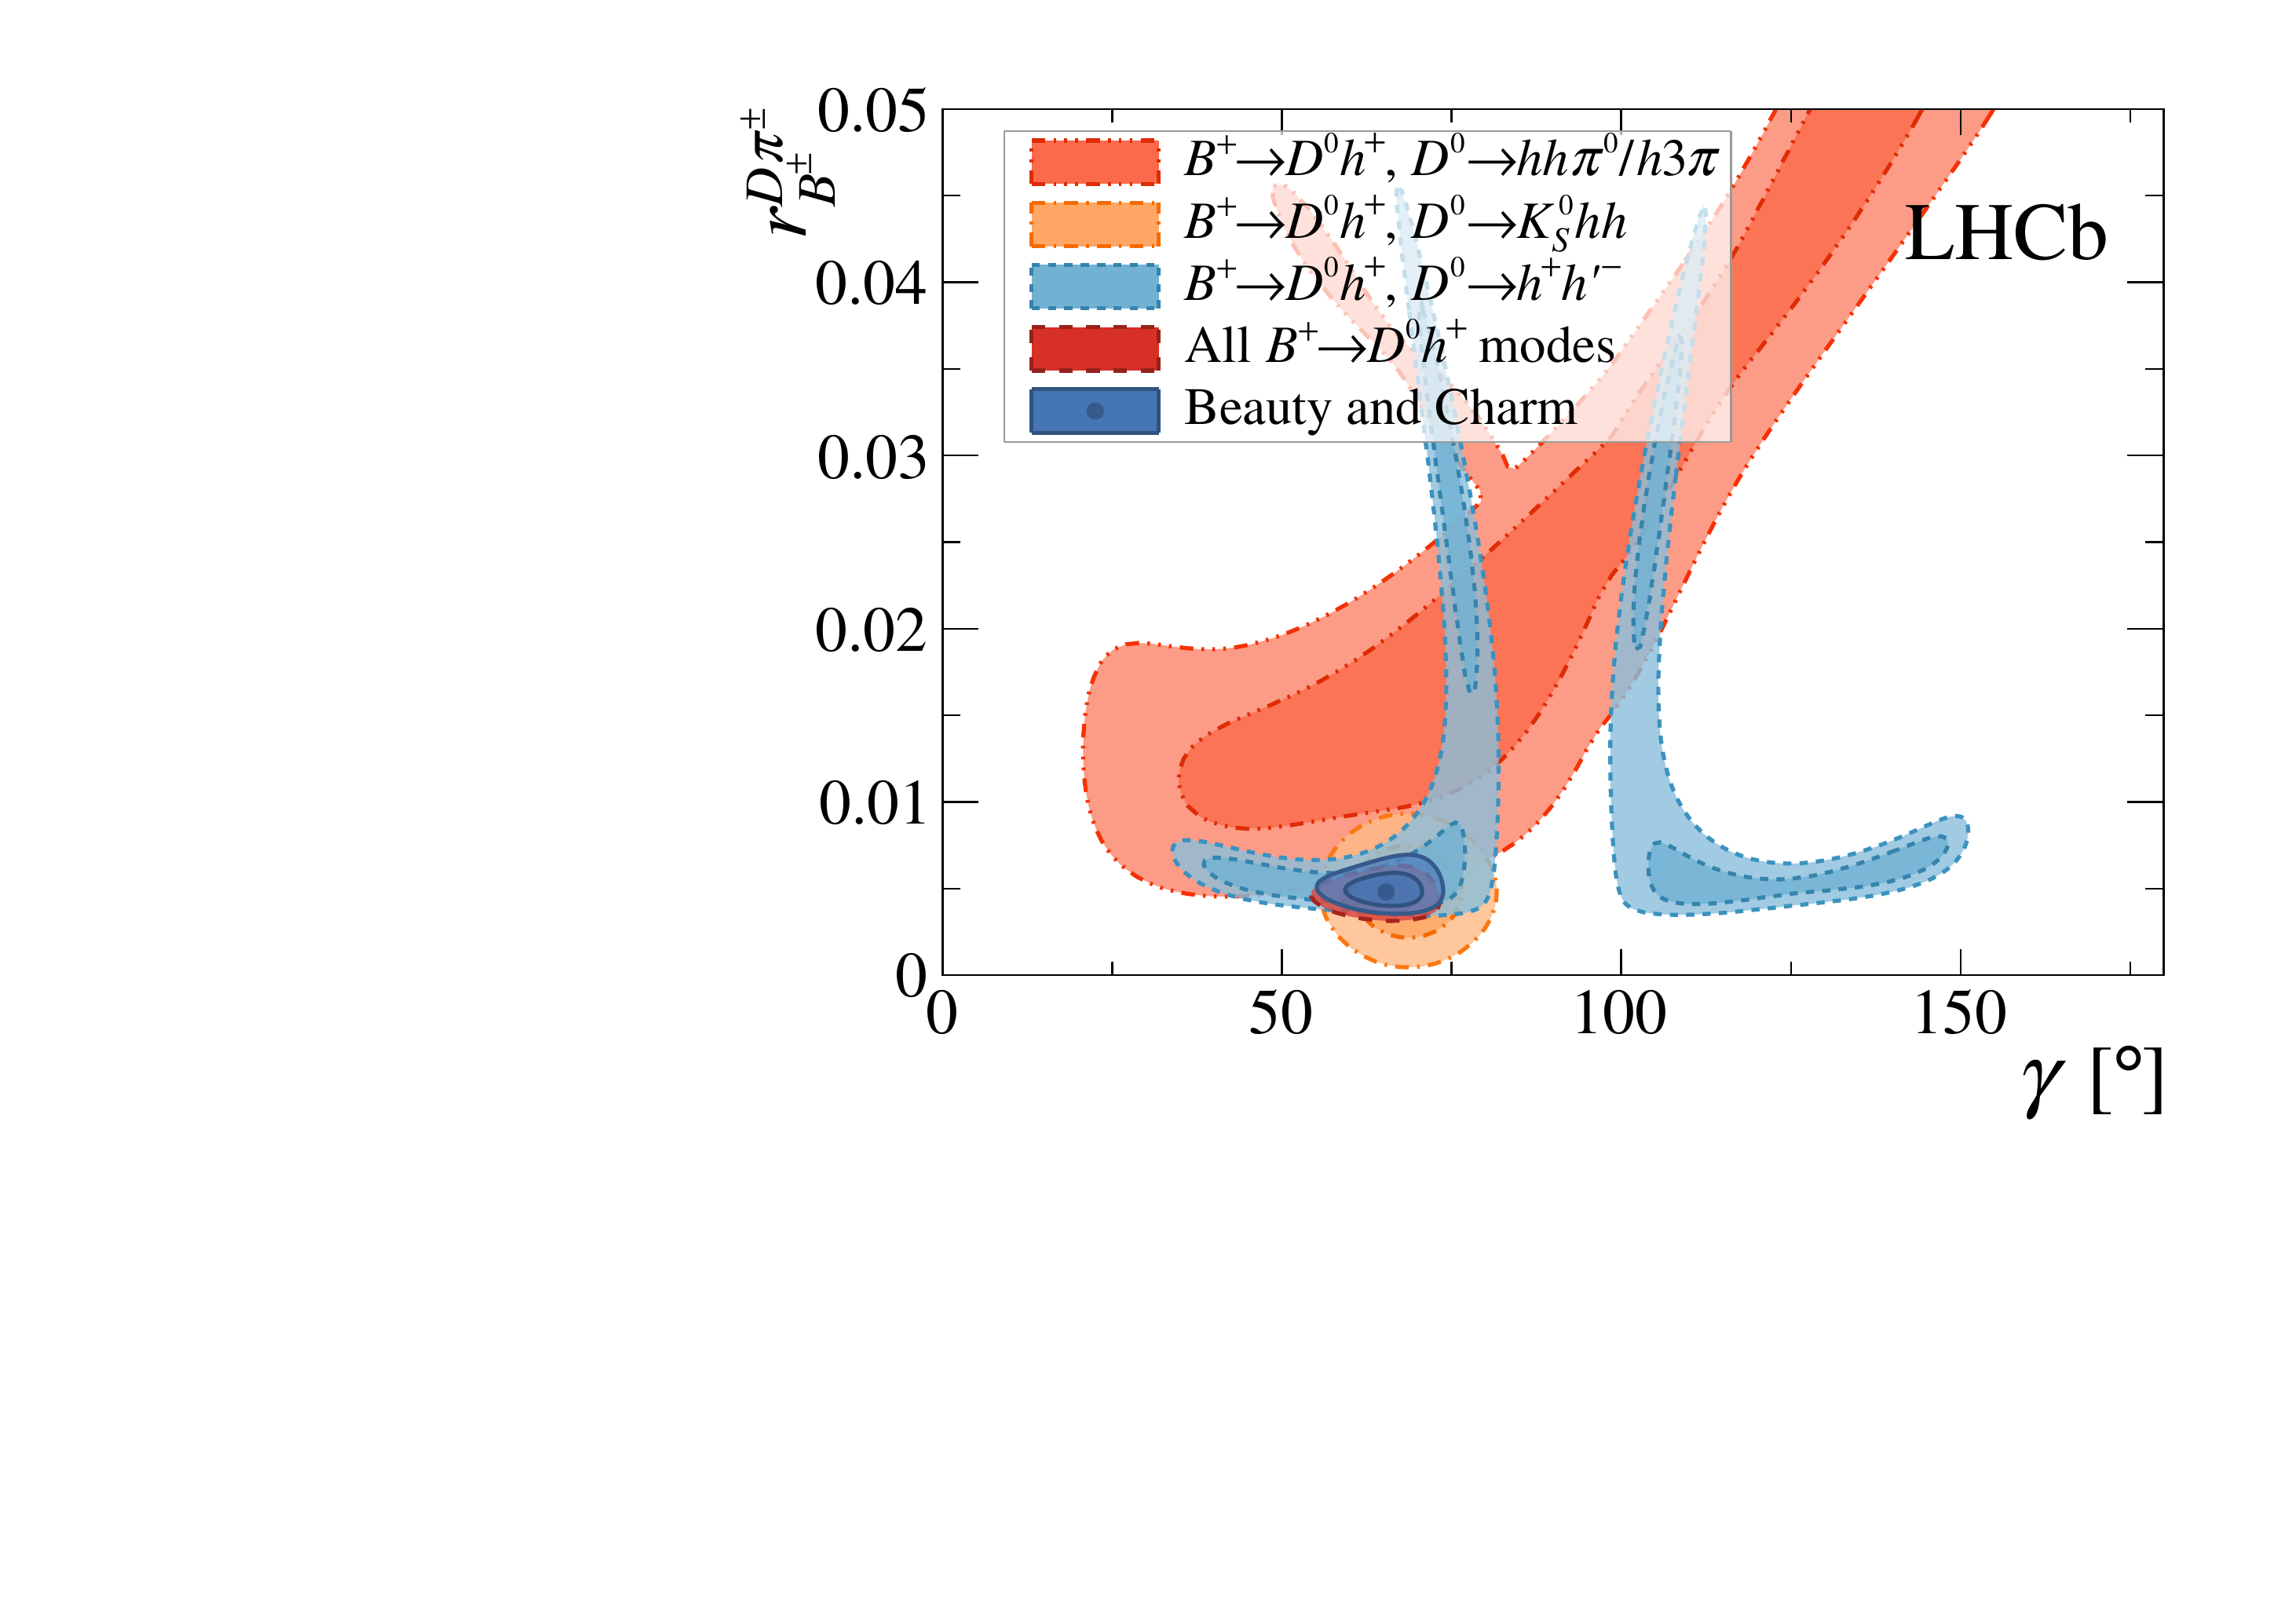}
  \includegraphics[width=0.48\textwidth]{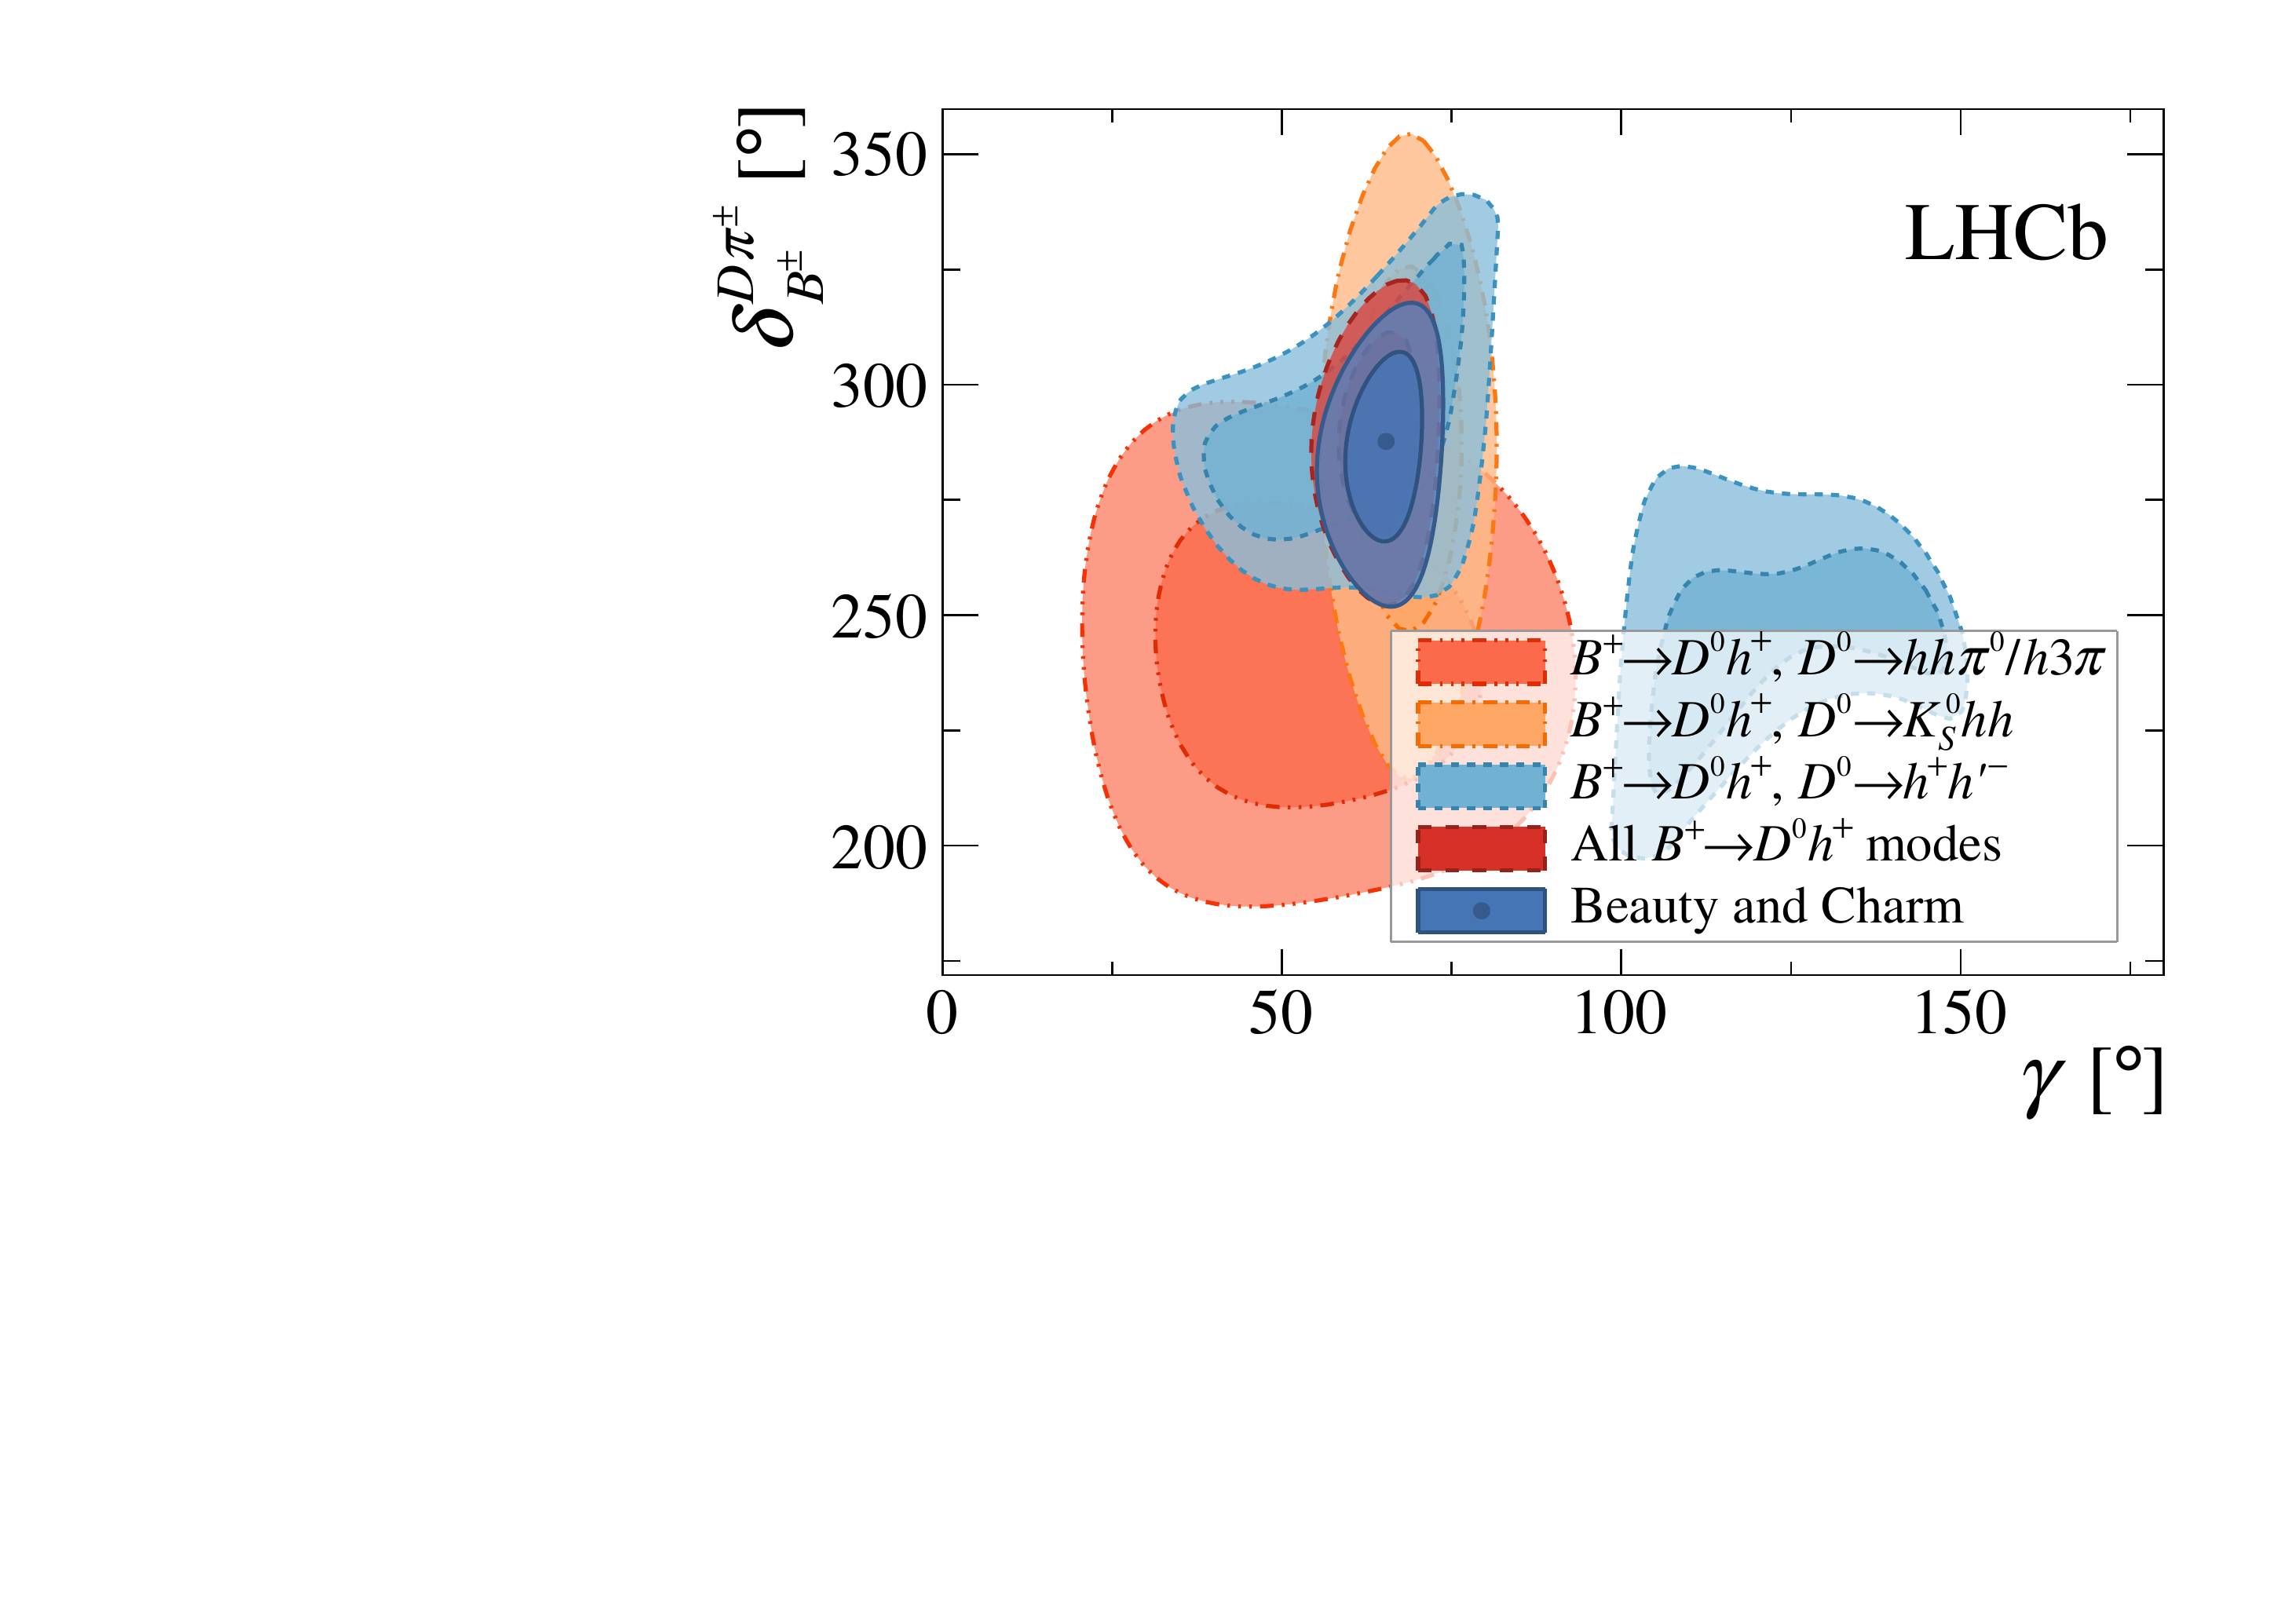}
  \includegraphics[width=0.48\textwidth]{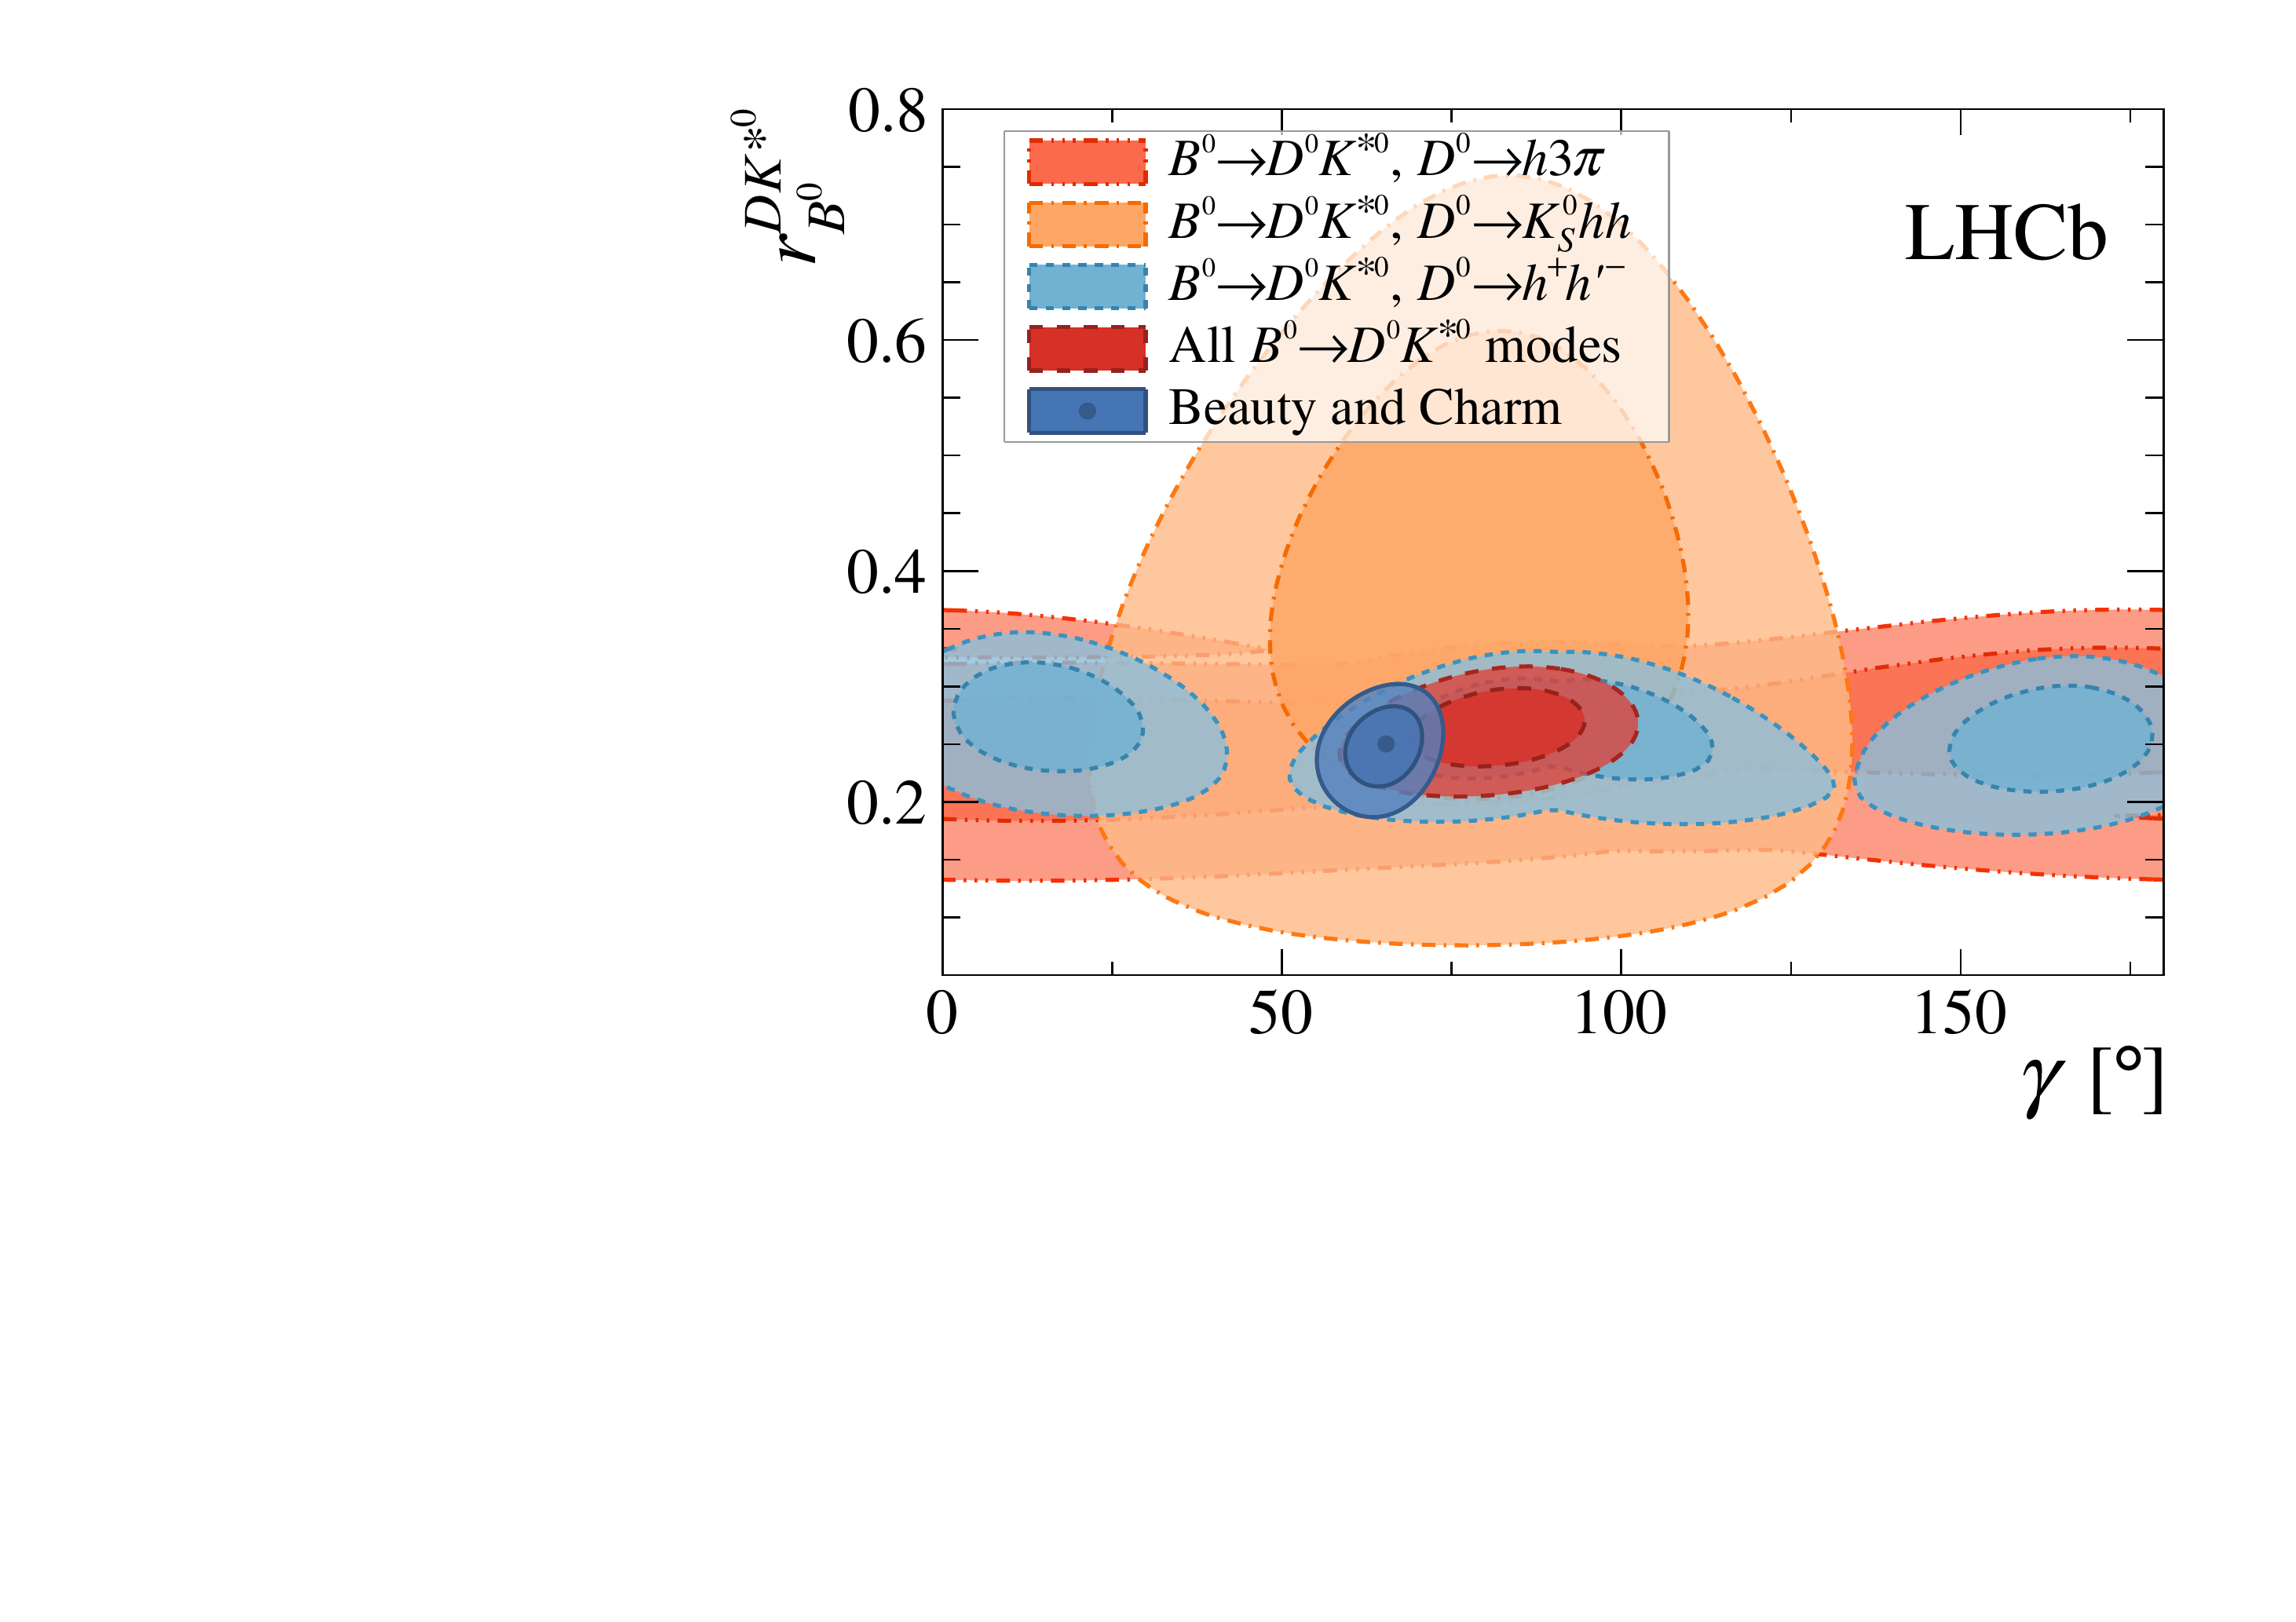}
  \includegraphics[width=0.48\textwidth]{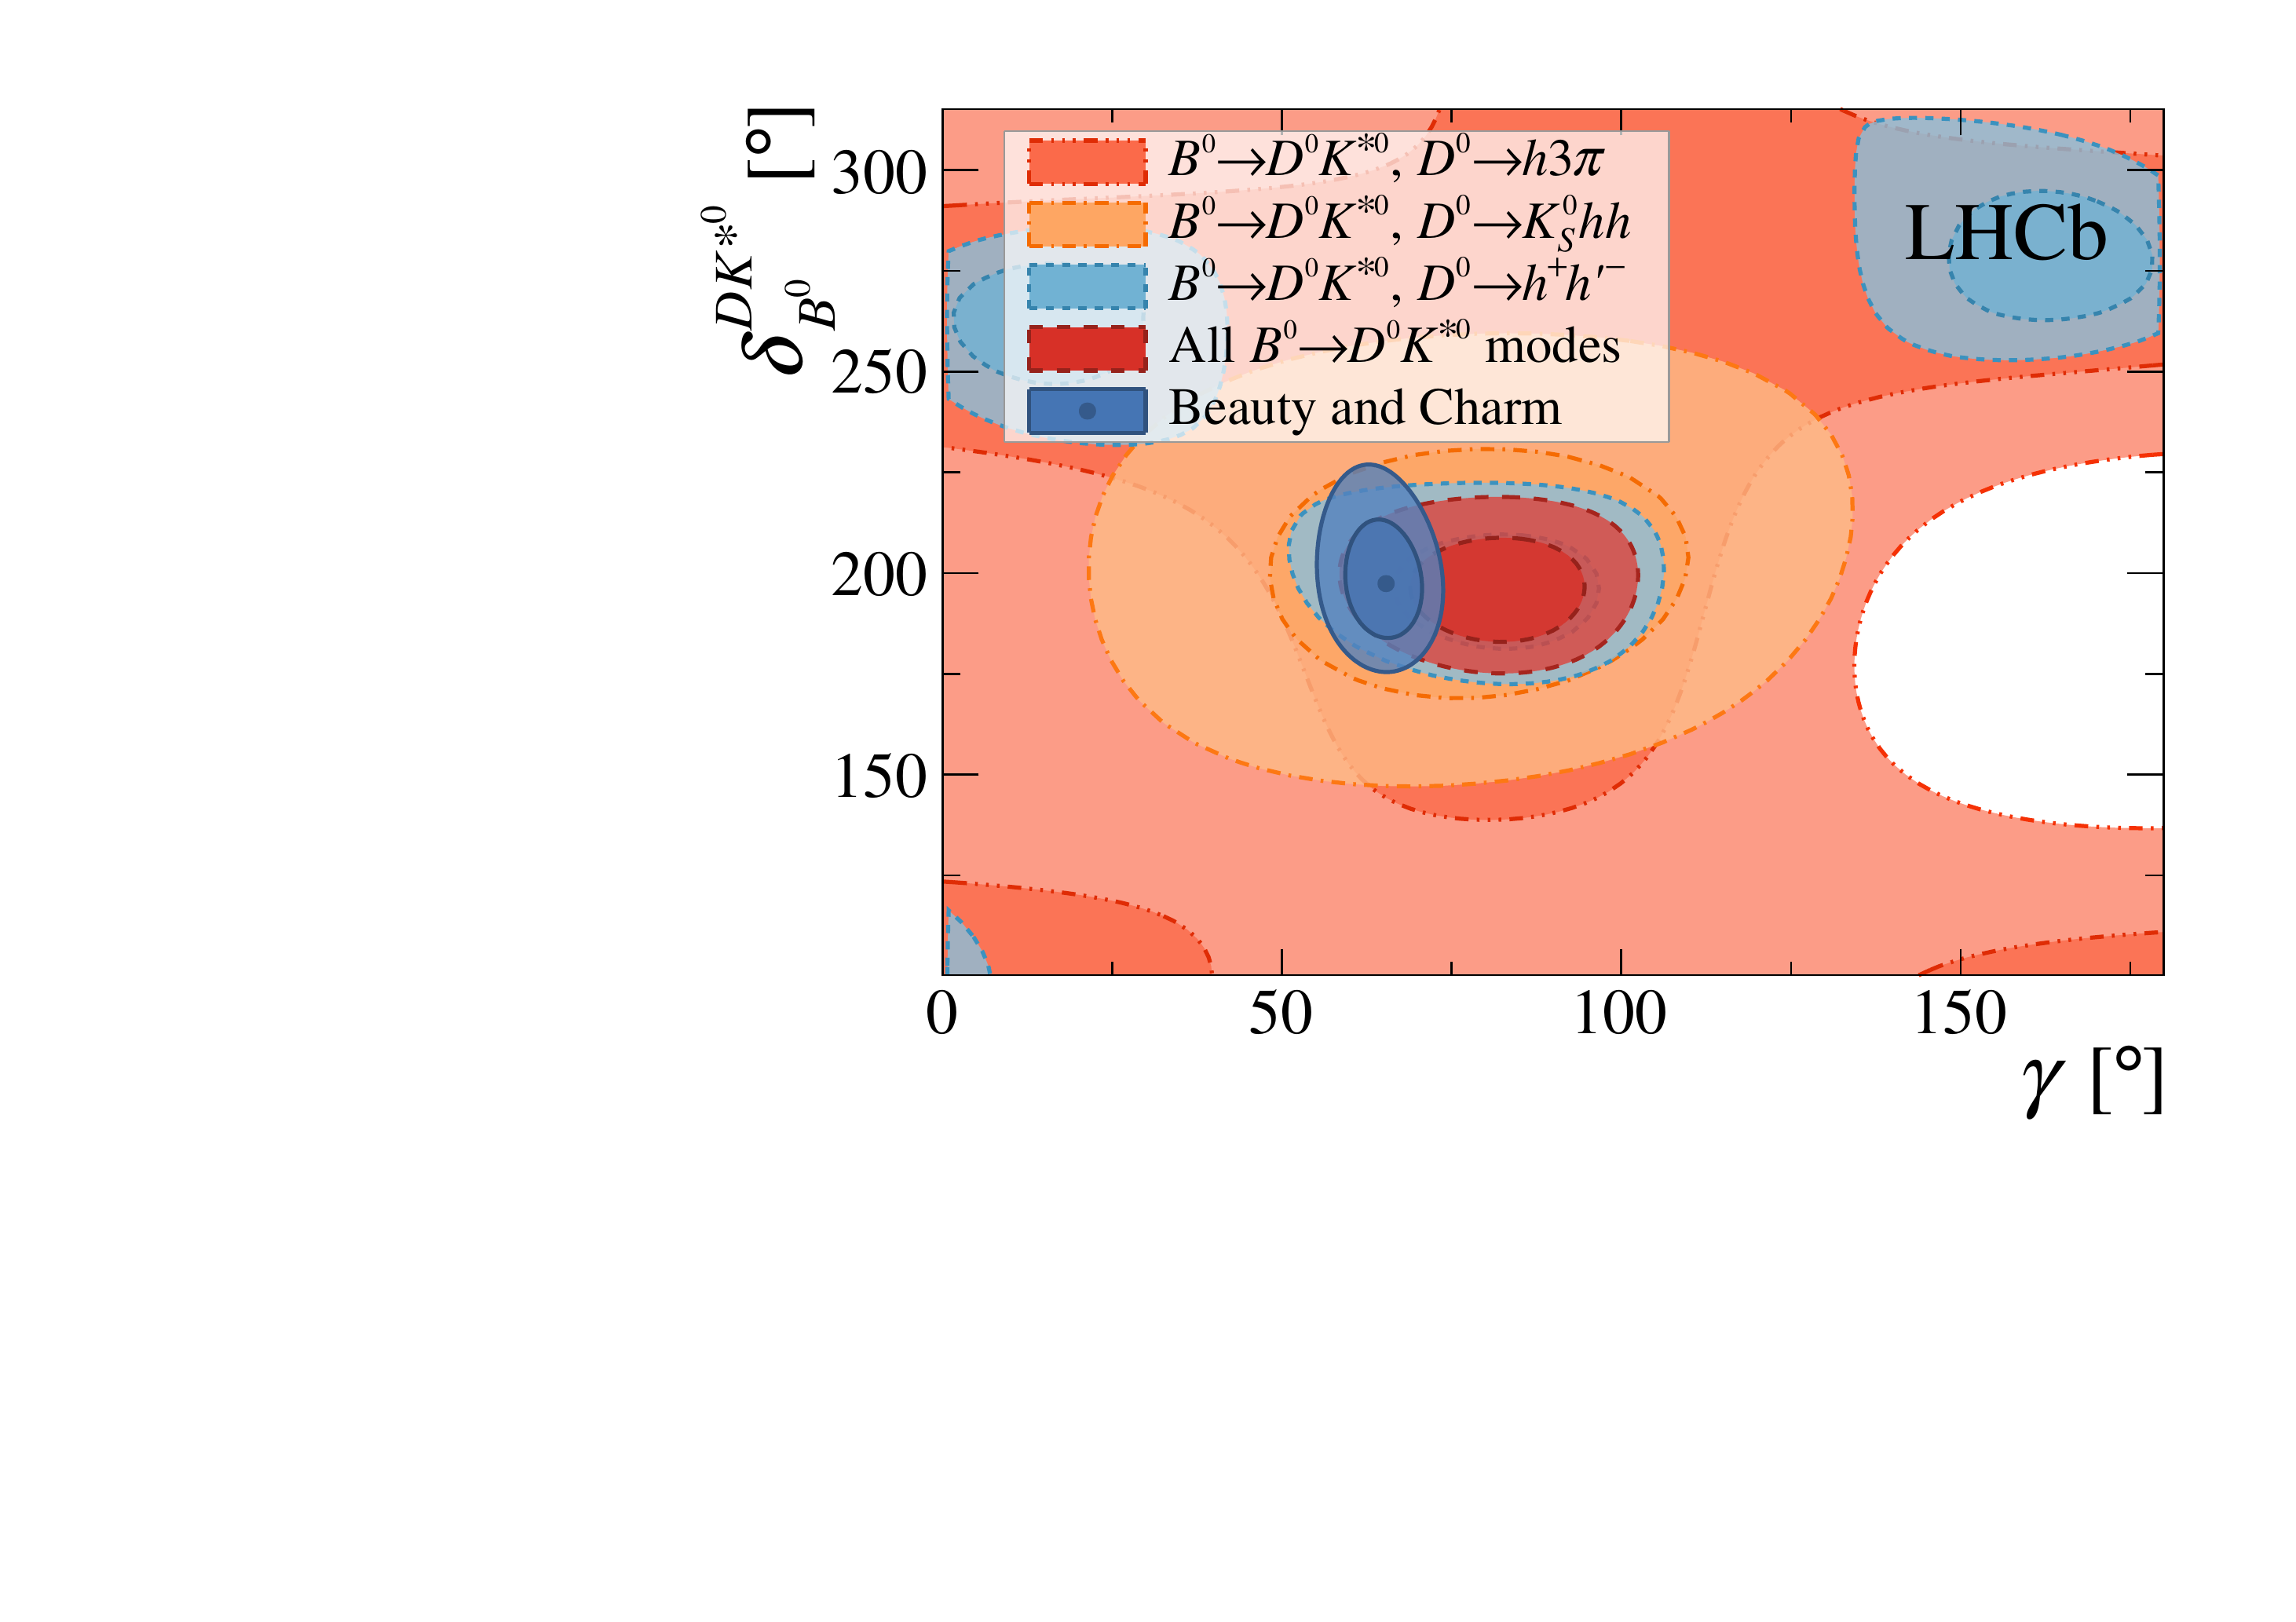}
  \caption{Profile likelihood contours for the components which contribute towards the \g part of the combination, showing the breakdown of sensitivity amongst different sub-combinations of modes.
  The contours are the two-dimensional $1\sigma$ and $2\sigma$ contours.}
  \label{fig:res:breakdown_2d_dh}
\end{figure}

\begin{figure}[!tb]
  \centering
  \includegraphics[width=0.9\textwidth]{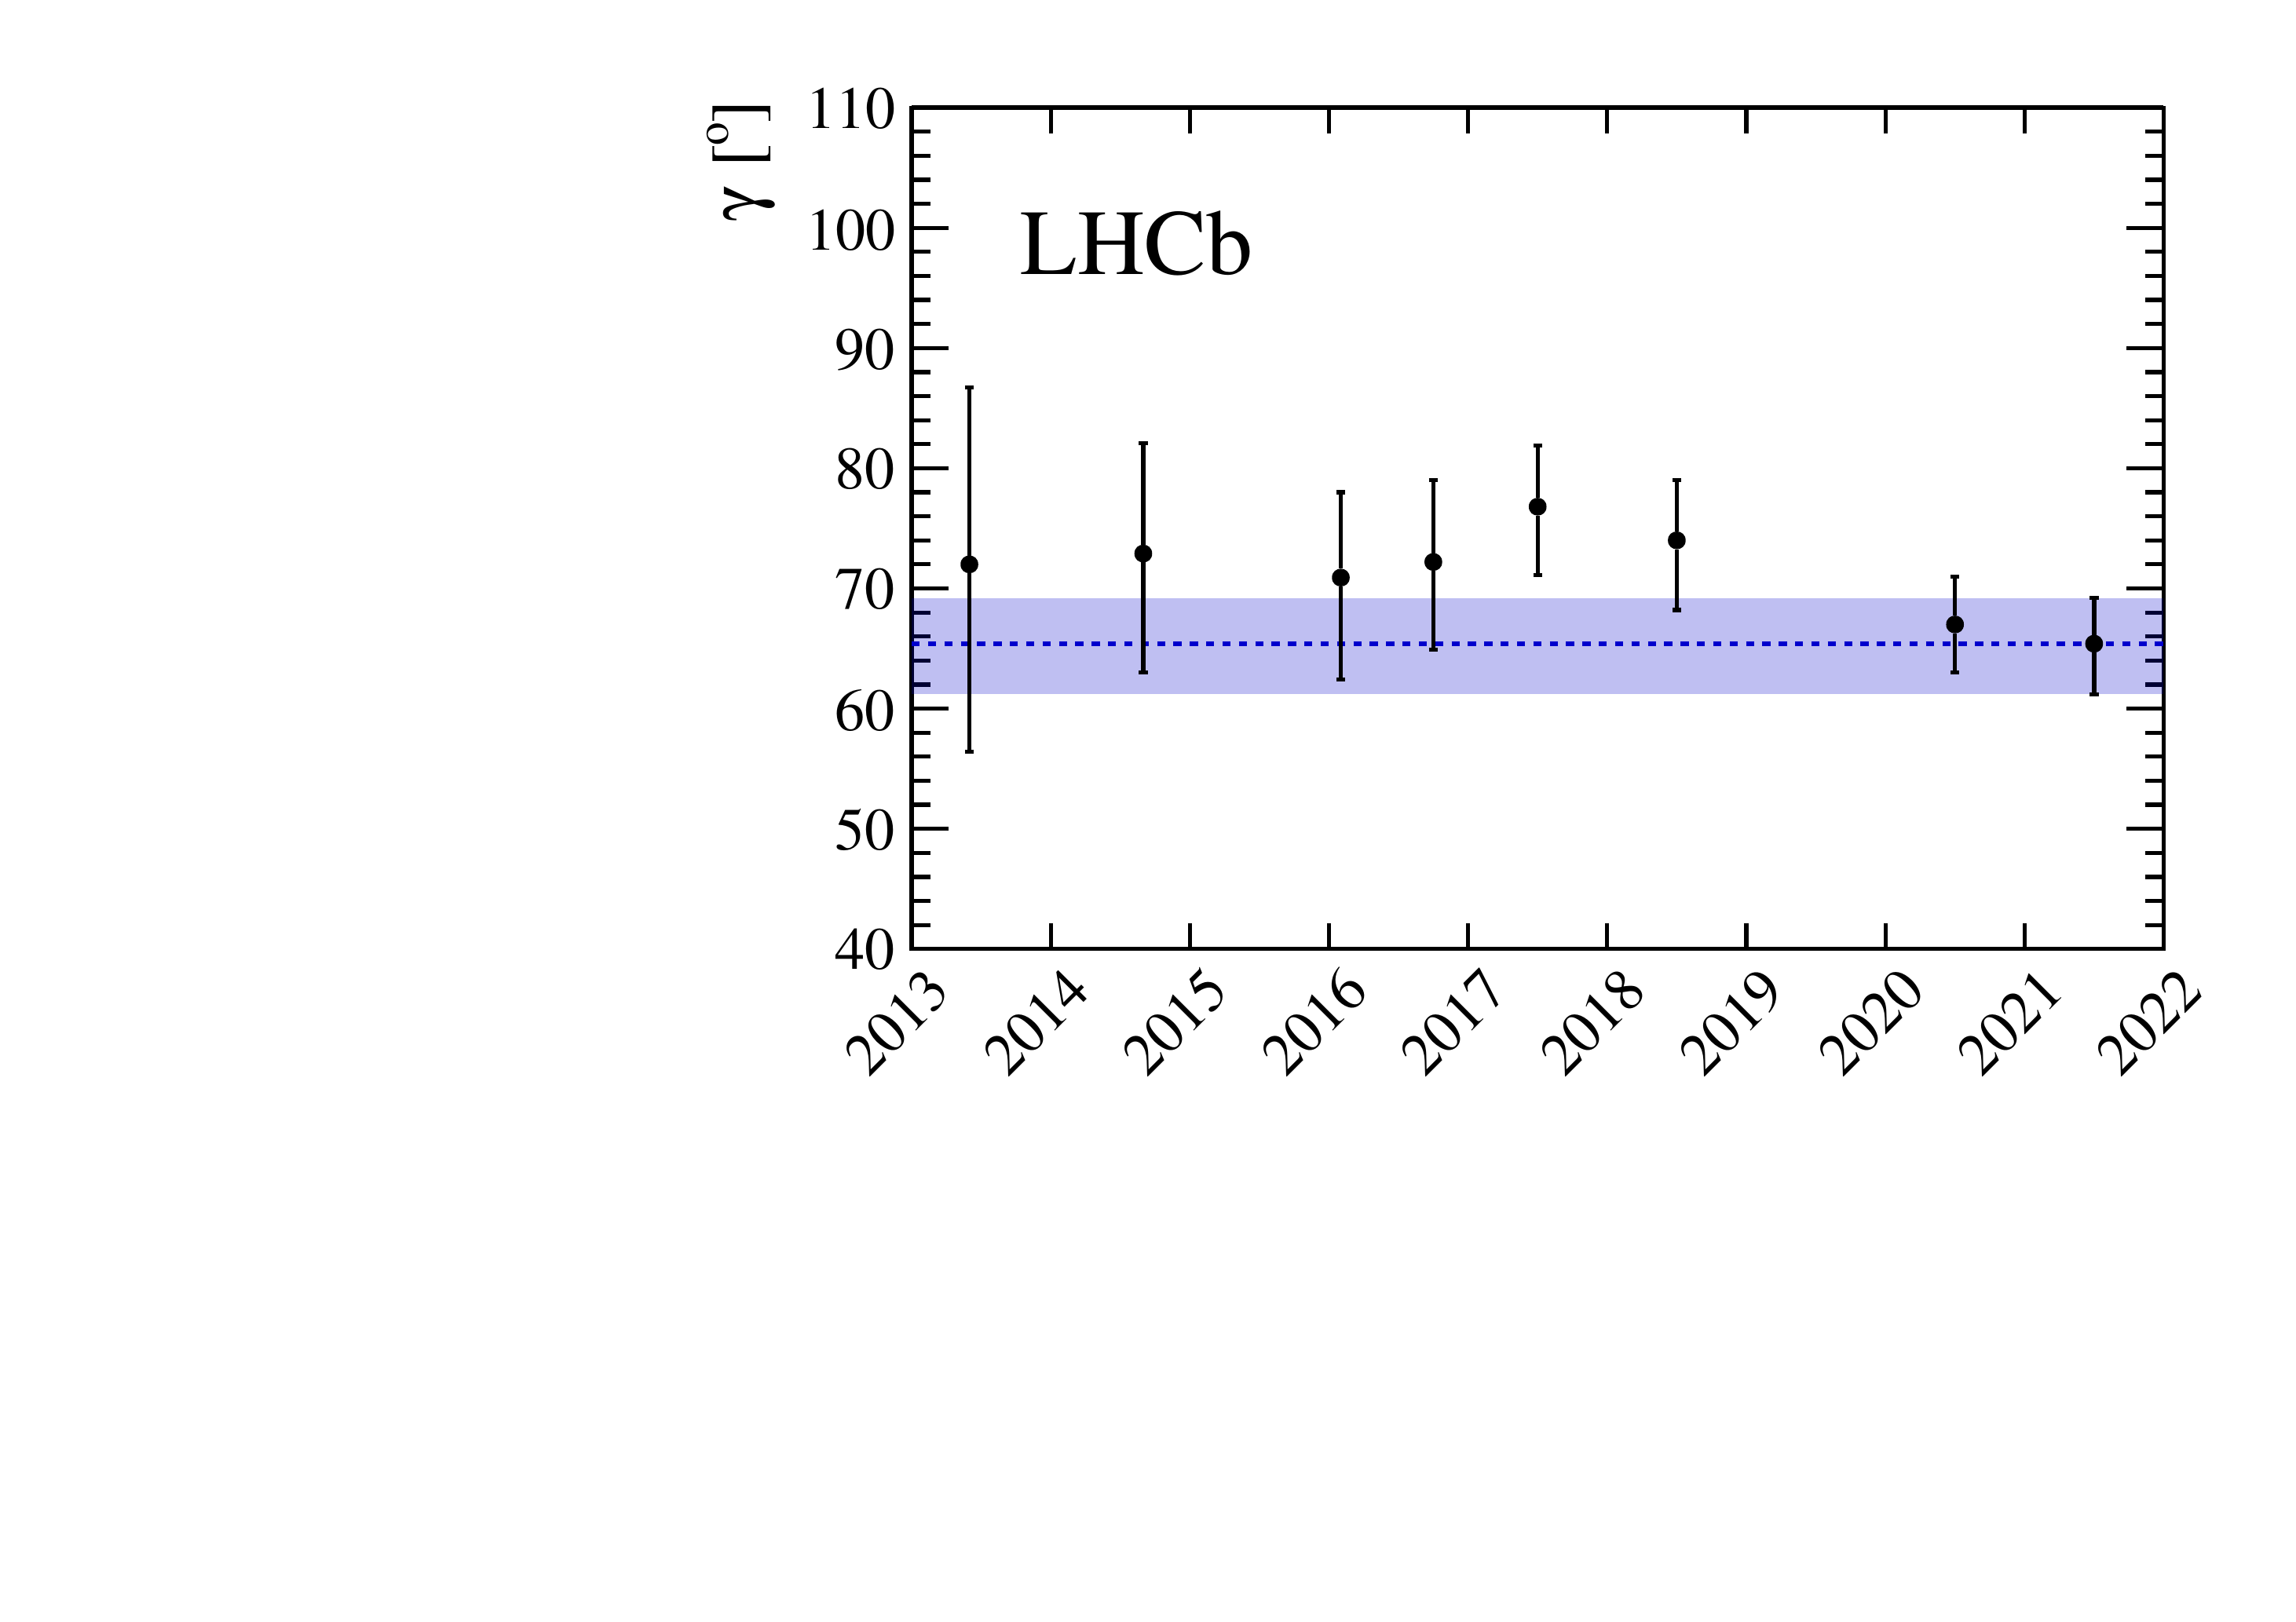}
  \caption{Evolution of the LHCb combination result for \g, with the central values and $1\sigma$ uncertainties in black, and the latest result and uncertainty highlighted by the dashed blue line and band respectively. }
  \label{fig:gammaevolution}
\end{figure}
